# Supplementary material for: Fingerprinting Search Keywords over HTTPS at Scale
Source: arXiv:2008.08161 source file (2020-08-18)
Supplement: Supplementary file 1 [file bootstrap_appendix_a.tex]

\begin{table}[H]
    \centering
    \caption{Classification accuracy (\%) with bootstrap enabled and disabled.}
    % \resizebox{0.8\linewidth}{!}{
    \begin{tabular}{l|cc}
        \hline
        & Enable Bootstrap & Disable Bootstrap \\ \hline
        \emph{PSC} & \\
        \emph{Wfin} & \\ 
        \emph{EtResp} & \\
        \emph{k-FP} &  \\
        \hline
        
    \end{tabular}
    % }
    
    \label{tab:bootstrap_accuracy}
\end{table}
